# Supplementary material for: A heterogeneously integrated lithium niobate-on-silicon nitride photonic platform
Source: arXiv:2112.02018 source file (2022-09-12)
Supplement: Supplementary file 1 [file SI.pdf]

# Supplementary information for "A heterogeneously integrated lithium niobate-on-silicon nitride photonic platform"

Mikhail Churaev[1*], Rui Ning Wang[1*], Viacheslav Snigirev[1*], Annina Riedhauser[2], Terence Blésin[1], Charles Möhl[2], Miles A. Anderson[1], Anat Siddharth[1], Youri Popoff[2,3], Ute Drechsler[2], Daniele Caimi[2], Simon Hönl[2], Johann Riemensberger[1], Junqiu Liu[1], Paul Seidler[2,†], Tobias J. Kippenberg[1,‡]

[1]*Institute of Physics, Swiss Federal Institute of Technology Lausanne (EPFL), CH-1015 Lausanne, Switzerland*

[2]*IBM Research - Europe, Zurich, CH-8803 Rüschlikon, Switzerland*

[3]*Swiss Federal Institute of Technology Zurich (ETH Zürich), CH-8092 Zürich, Switzerland*

*These authors contributed equally to this work

Emails: ‡ tobias.kippenberg@epfl.ch, † pfs@zurich.ibm.com

## CONTENTS

I. Fabrication details 2

II. Linewidth histograms for wafer map 3

III. Fiber-to-chip transmission calibration 3

IV. Electro-optic efficiency 4

V. Bending losses 5

VI. Electro-optic microring characterization 6

VII. Electro-optic frequency comb simulation 6

VIII. Supercontinuum and second-harmonic generation in hybrid waveguides 7

Supplementary Table 1 9

References 10

# I. FABRICATION DETAILS

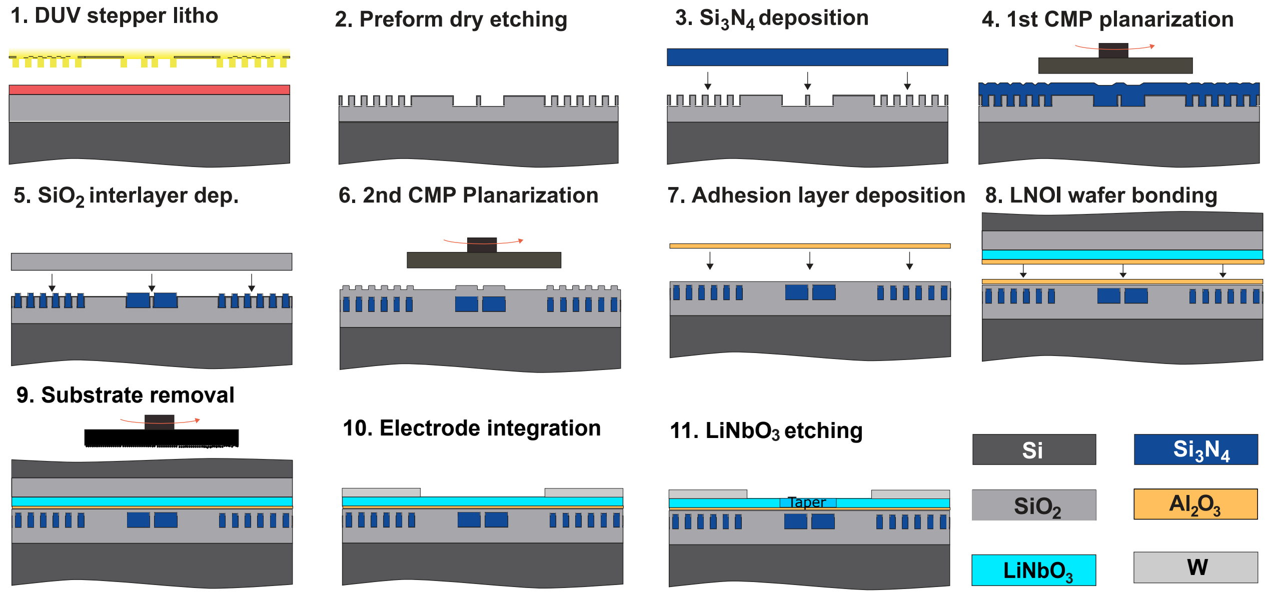


**Supplementary Figure 1:** Schematics of all the processing steps involved in fabrication of our heterogeneously integrated $LiNbO_3$ photonic circuits. Steps 1-5 correspond to standard Photonic Damascene process, steps 6-9 are related to surface preparation and bonding, and 10-11 are the post-bonding processing.

Fabrication steps 1-4 in figure S1 are described in detail elsewhere [1]. After the first chemical-mechanical polishing (CMP) process, the surface is not yet ready for wafer bonding: In order to clean the silica particles from the CMP slurry, a short dip in buffered hydrofluoric acid (BHF) is performed. This generates some topography between the silicon nitride structures and the surrounding silicon oxide cladding. To obtain a bonding-ready surface, an interlayer of a few hundred nanometers of silicon oxide is deposited by LPCVD and subsequently polished down and planarized. As described in the main text, after this step, the roughness and long-range non-uniformity are low enough for bonding. The remaining interlayer thickness is about 100 nm. Moreover, reflectometry measurements revealed that the thickness variation of the interlayer was of about 5 nm over the whole wafer.

In order to bond with the lithium niobate on insulator (LNOI) wafer, the surface of both wafers is cleaned, and a thin alumina layer of a few nanometers is deposited with atomic layer deposition (ALD) on both of them. The wafers are then brought into contact. To increase the bonding strength, the bonded wafers are annealed for several hours at 250C. After bonding, the Si of the LNOI carrier is removed by grinding and TMAH (tetramethylammonium hydroxide). The buried oxide of the LNOI carrier is removed with buffered hydrofluoric acid. Tungsten is then sputtered onto the bonded lithium niobate and patterned into electrodes with fluorine-based reactive ion etching (RIE).

The next step is to pattern the bonded lithium niobate thin film. The objective here is two-fold: remove the LN from the chip facets and fabricate LN tapers to ensure a smooth transition in the waveguide as discussed in the main text. To this end, a $SiO_2$ protection layer is first sputtered on the LN surface. Ion beam etching is then employed with a photoresist etch mask to etch both the $SiO_2$ protective layer and the $LiNbO_3$, leaving only a very thin slab of less than 50 nm. The etching is performed with an Argon ion beam impinging at an angle of 30° while the wafer is rotating. In order to reduce the accumulation of re-sputtered material during etching, the photoresist mask is reflown at 130°C for 3'30" after exposure and development. After etching and removal of the photoresist, the re-sputtered materials are removed by wet etching in a concentrated solution of ammonia and hydrogen peroxide heated to 85°C. During this cleaning, the surface of the LN thin film is protected by the $SiO_2$ layer. After cleaning, the $SiO_2$ layer can be removed using a bHF solution. In this process step, the thin remaining LN slab acts as a protective layer to prevent the HF from etching the interlayer of the silicon nitride device wafer and undercutting the LN tapers.

To release the chips, the edges are defined by dry-etching the silicon oxide cladding with fluorine-based chemistry, and then further down into the Si carrier using the Bosch process. This ensures a relatively smooth chip facet that does not require further polishing. The chips are then separated by grinding the wafer down to the etched depth from the backside.

## II. LINEWIDTH HISTOGRAMS FOR WAFER MAP

Fig S2 shows the $\kappa_0/2\pi$ histograms for the same 21 GHz FSR microring resonator, measured in 5 different fields on the bonded 2" wafer. The most probable values for each field are given in Fig 2(e) of the main manuscript.

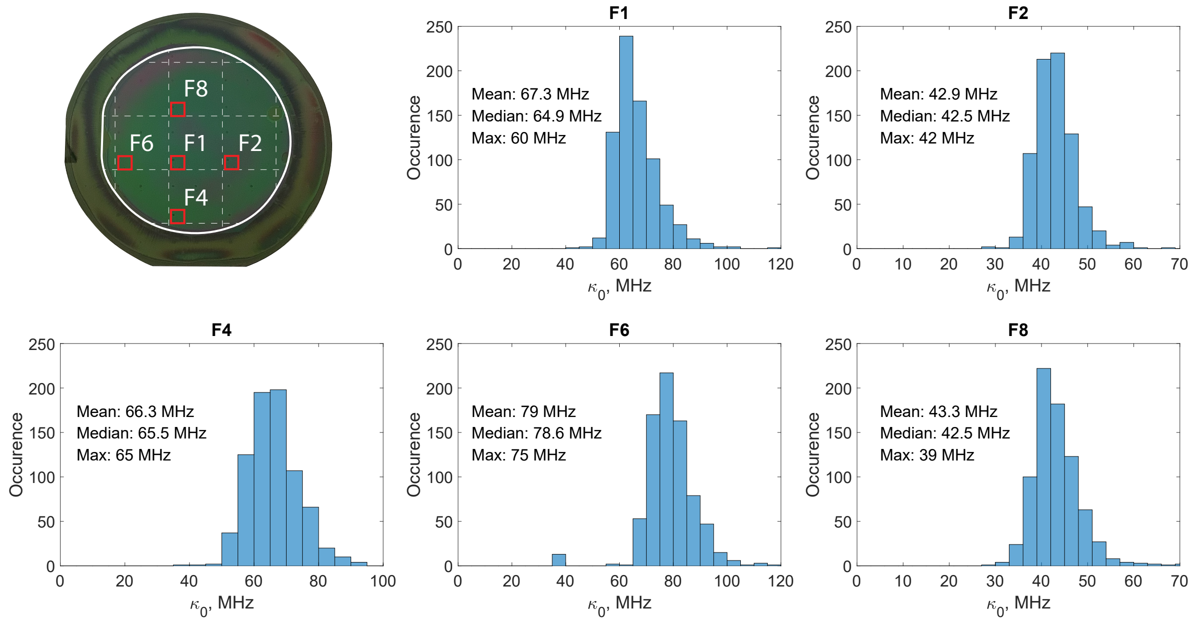


**Supplementary Figure 2:** Linewidth data for the wafer map presented in the main text.

## III. FIBER-TO-CHIP TRANSMISSION CALIBRATION

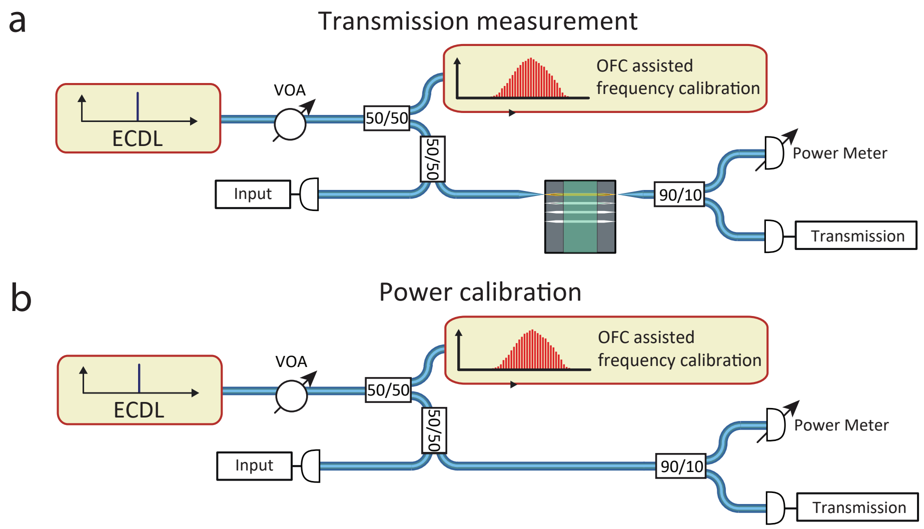


**Supplementary Figure 3:** Layout of fiber-to-fiber transmission measurement setup (a) and power calibration (b). ECDL - external cavity diode laser, OFC - optical frequency comb, VOA - voltage-controlled attenuator.

The absolute fiber-to-fiber transmission measurements are done in two steps as depicted in Figure S3. In the first step we couple into the chip with lensed fibers and record the transmission using a photodetector (marked as

"transmission"). To eliminate any uncertainty in ECDL power we split the signal and track it directly, using an additional photodiode marked as "input". Then we connect the input and output arms of the setup directly using a fiber patch cord. By recording the same metrics for a directly connected patch cord we are able to normalize the photonic chip transmission measurements. The OFC-assisted frequency calibration is described elsewhere [2].

## IV. ELECTRO-OPTIC EFFICIENCY

In our work we use 950 nm thick silicon nitride waveguides, and keep an interlayer silicon dioxide layer of about 100 nm thickness. The waveguide width ranges from 1.7-2.0 $\mu$m. The X-cut LNOI wafer used in the work is provided by NanoLN, having 300 nm thickness. After processing the thickness was reduced to 275 nm. The corresponding cross-section and optical mode distribution are depicted in Figure S4(a).

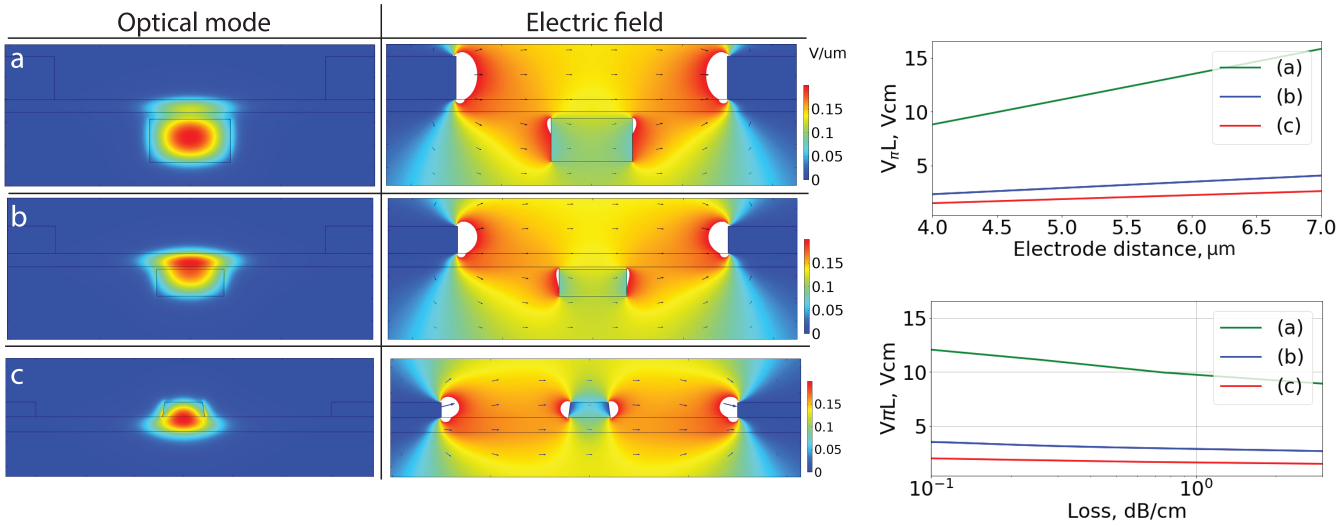


**Supplementary Figure 4:** Comparison of electro-optic efficiency for 3 different structures: (a) the bonded lithium niobate structure presented in this work and (b) the bonded structure with optimized geometry for electro-optic modulation. (c) typical ridge waveguide configuration. The plots on the right show simulation results for the half-wave voltage - length product ($V_\pi L$) for a MZM configuration and the corresponding accumulated linear loss due to the metal presence. White parts in electric field distribution correspond to areas with a saturation of electric field larger than 0.2 V/$\mu$m.

The main figure of merit for electro-optic modulation is the half-wave voltage - length product ($V_\pi L$) value. To compare electro-optic efficiency for classical ridge waveguides [3, 4] and the hybrid structure presented in this work we perform FEM simulations in COMSOL Multiphysics for optical mode and electrostatic field distribution. The refractive index change under external modulation electric field $E$ is:

$$\Delta n_{\text{eo}} = \frac{1}{2} n^3 r_{33} E.$$

Here we consider both modulation electric field $E$ and optical electric field $E_{\text{opt}}$ to be coplanar with extraordinary $LiNbO_3$ crystal axis. The modulation electric field strength $E$ is linearly proportional to the voltage applied on the electrodes so that $E = V/d_{\text{eff}}$, where effective distance value $d_{\text{eff}}$ represents just a linear scaling parameter. We calculate this parameter by simulating electrostatic and optical fields with 1V applied to the electrodes. The effective distance will be then inverse proportional to the normalized effective electric field, taking into account optical and electrostatic field overlap:

$$d_{\text{eff}} = \frac{1V}{E_{\text{eff}}};\ E_{\text{eff}} = \frac{\int_{\text{LN}} |E_{x,\text{opt}}|^2 E_{x,\text{el}} dS}{\int |E_{x,\text{opt}}|^2 dS}$$

We calculate the $V_\pi L$ values for dual-arm Mach-Zehnder modulators as [5]:

$$V_\pi L = \frac{\lambda d_{\text{eff}}}{2n^3 r_{33}},$$

where $\lambda$ is the optical wavelength.

The $V_\pi L$ value depends on the gap distance between the electrodes, so to compare the overall electro-optic efficiency we need to also take into account optical losses induced by the metal electrodes which limits the minimum electrode gap. In Figure S4 we give a comparison of half-wave voltage-length products as a function of induced optical loss for the current structure, optimized bonded structure, and classical ridge waveguide structure. As can be seen from the simulations, the bonded structure slightly compromises electro-optic efficiency ($\times 2$ factor) primarily because of weaker optical mode confinement (therefore induced mode area). As was discussed in the main text, the hybrid waveguide conceptually behaves as a ridge waveguide since in case of a ridge waveguide the electric field avoids the waveguide itself and is accumulated in the slab (see Figure S4(c) electric field distribution). Case (b) corresponds to a 1 $\mu$m wide waveguide having 600 nm thickness and 100 nm interlayer thickness bonded to a 300 nm thick lithium niobate slab. In this configuration, the mode confinement in $LiNbO_3$ reaches 40%.

## V. BENDING LOSSES

We perform numerical FEM simulations to verify if the "electro-optic" configuration discussed in the previous section is not dominated by whispering-gallery losses (bending losses). The high optical mode participation in lithium niobate could lead to significant radiation into the slab at waveguide turns. However, according to our simulations (cf. Figure S5(a)), it is possible to achieve high quality factors ($>10^7$) for microresonators having down to 100 $\mu$m radius with 40% of the mode sitting in lithium niobate. The critical point here is to minimize the silicon oxide interlayer (spacer) thickness. In the case of a thick spacer, the optical mode starts to split into high-confinement core mode and low-confinement slab mode, which leads to a large dissipation of the latter at waveguide turns (see Figure S5(b)). Unfortunately, the interlayer spacer cannot be removed fully, as it provides a flat bonding-ready surface for our hybrid structure, but for future high-participation applications, its thickness should be minimized for better performance.

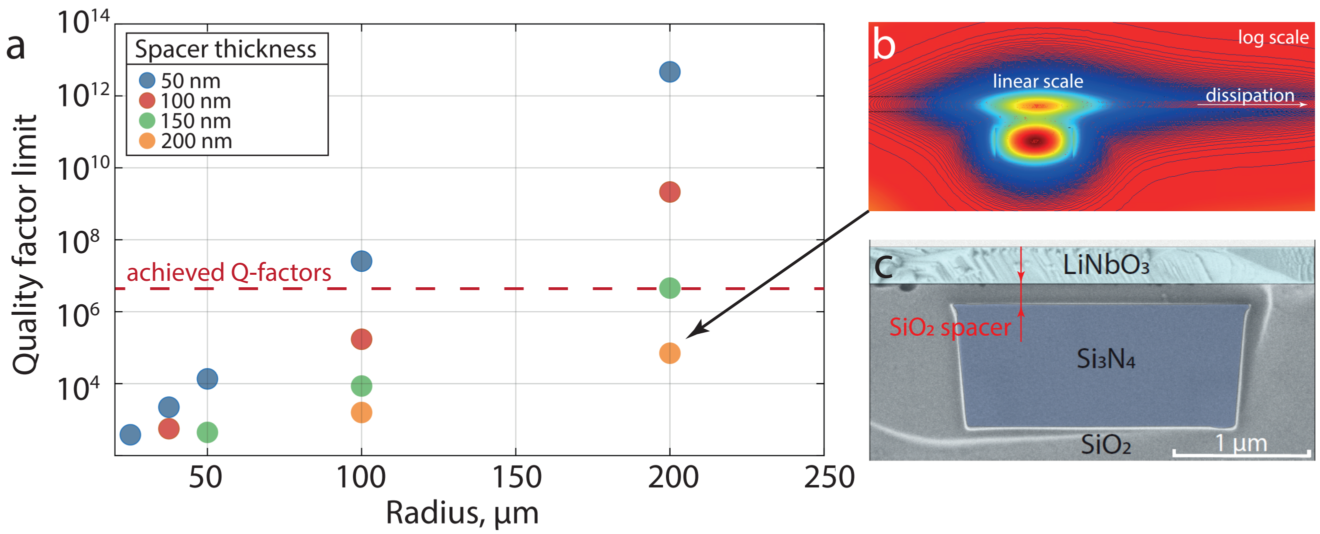


**Supplementary Figure 5:** Numerical simulations (FEM) of bending loss-limited Q-factors in hybrid waveguides. (a) Simulation results for the "electro-optic" waveguide geometry discussed in the previous section for different bending radii and spacer thicknesses. (b) Example of an optical mode dissipation in case of a thick spacer. The inner waveguide colors display linear-scale mode distribution, while the far-field lines are in log scale to visualize an optical mode dissipation in the tail, being de-coupled from the $Si_3N_4$ waveguide core. (c) Cross-section of a typical waveguide used in this work with an indication of the spacer.

## VI. ELECTRO-OPTIC MICRORING CHARACTERIZATION

The linear tuning of the 20 GHz hybrid device is measured by locking the CW laser on a resonance of the microresonator via a PDH stabilization as shown in figure S6. A 30 Volts peak-to-peak ramp signal is applied on the electrodes of the device and the PDH error signal is obtained by phase-modulating the pump laser (at a frequency in the range of 500 – 800 MHz) before coupling to the cavity, using an electro-optic modulator (EOM, iXblue MPX-LN-0.1). The modulated signal is detected after the resonator and demodulated to DC using the same RF signal. After demodulation, the baseband signal is low-pass-filtered and sent to a PID servo-controller (Toptica FALC). The servo output is then measured and processed after due calibration to estimate the linear tuning coefficient of the device as 41.69 MHz/V.

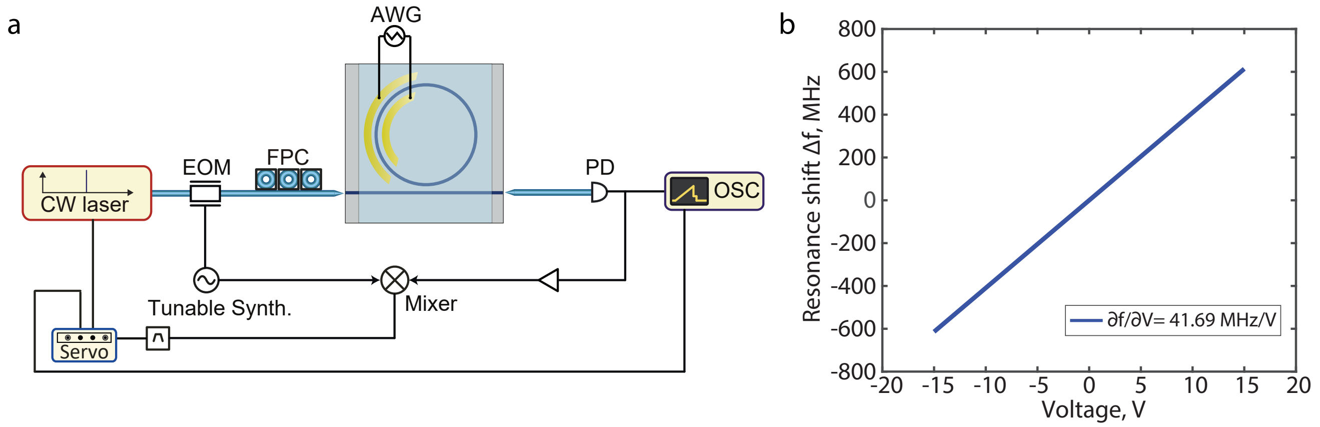


**Supplementary Figure 6:** Linear resonance tuning measurements. a) Experimental schematic of linear tuning measurement via Pound-Drever-Hall laser stabilization method. The CW laser is locked to the microresonator resonance and on applying an electrical signal on the electrodes, the calibrated servo output provides the linear tuning coefficient of the device under test. b) Resonance shift versus applied voltage for a 21 GHz FSR resonator. The linear tuning coefficient at DC is $\Delta f/V$ = 41.69 MHz/V.

The metal electrodes essentially form a capacitive element. The value of the associated capacitance is an essential information to characterize the modulation efficiency of traveling-wave devices, and the single electro-optic coupling of resonant ones. Since the microwave response of $LiNbO_3$ is populated by piezoelectric features and the low frequency response is modified by the probes, the static capacitance is obtained here by taking the slope of the imaginary part of the admittance at high frequencies. The admittance is obtained from a microwave reflection measurement

$$Y_{11} = \frac{1}{Z_0}\frac{1 - S_{11}}{1 + S_{11}} \tag{1}$$

for 1-port devices, with a characteristic impedance $Z_0 = 50\Omega$ [6].

We measure the capacitance of 3 types of devices: 20 GHz, 50 GHz, and 100 GHz FSR microresonators with electrodes (cf Figure S7). The decreasing capacitance for higher FSR resonators is in a good agreement with the corresponding electrode length dependency.

## VII. ELECTRO-OPTIC FREQUENCY COMB SIMULATION

In the electro-optic frequency comb experiment presented in Fig 3(c) of the main manuscript we use the RF power of 40 dBm at $\Omega_{\mathrm{mw}}$=21 GHz frequency. According to the microwave characterization (see section S4), the electrode capacitance is around 1200 fF. The applied voltage amplitude can be calculated as:

$$V_p = \sqrt{\frac{2P_{\mathrm{mw}}}{C\Omega_{\mathrm{mw}}}},$$

where $\Omega_{\mathrm{mw}} = 21\mathrm{GHz}$ is the microwave frequency applied. Which gives us $V_p \approx 40\mathrm{V}$.

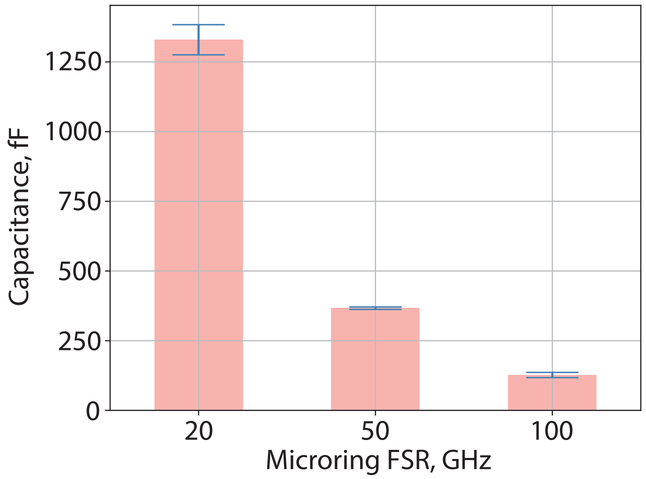


**Supplementary Figure 7:** Measured capacitance for 3 types of microresonator electrode pairs. The error bars show distribution over an average value.

Now, knowing the linear tuning of the resonator $\partial\nu/\partial V = 41\text{MHz/V}$ (cf section S4) one can calculate the electro-optic coupling rate $\Gamma_{\text{mw}}$ as:

$$\Gamma_{\text{mw}}/2\pi = V_{\text{p}} \times \partial\nu/\partial V \approx 1.5\text{GHz}$$

Full free spectral range resonance shift (21 GHz) would correspond to an intra-cavity electro-optic phase shift of $2\pi$. Therefore the phase modulation amplitude can be estimated as:

$$\beta = \frac{\Gamma_{\text{mw}}}{\text{FSR}} \approx 0.14\pi$$

For the simulations we consider an optical ring coupled to a bus waveguide with external coupling rate $\kappa_{\text{ex}} = 16$ MHz and internal loss rate $\kappa_0 = 65$ MHz. The values are taken from linear optical measurements. The cavity is excited by a monochromatic laser with photon flux $s_{\text{in}} = P/\hbar\omega_p$ (P is the input power) and frequency $\omega_p$, which is close to resonance frequency $\omega_0$. In the experiment we keep the pump on resonance ($\omega_p = \omega_0$) however some deviations might appear due to the thermal shifts of the resonance under high microwave power. The corresponding linear equation of motion for the slowly varying mode amplitude $b_\mu$ can be written as:

$$\partial_t b_\mu + (\frac{\kappa_{\text{ex}}}{2} + \frac{\kappa_0}{2})b_\mu + i(\omega_0 - \omega_p)b_\mu = \sqrt{\kappa_{ex}} s_{\text{in}} \delta_{\mu,0}$$

Under electro-optic modulation, the neighboring cavity modes start to couple with a coupling rate $\Gamma_{\text{mw}}$. Taking the electro-optic coupling into account, we derive the following coupled mode equation analogically to [7]:

$$\partial_t b_\mu + (\frac{\kappa_{\text{ex}}}{2} + \frac{\kappa_0}{2})b_\mu + i(\omega_0 - \omega_p)b_\mu = \sqrt{\kappa_{ex}} s_{\text{in}} \delta_{\mu,0} + i\frac{\Gamma_{\text{mw}}}{2}(b_{\mu+1} + b_{\mu-1})$$

As discussed in the main text the group velocity dispersion ($D_2$) is measured to be small compared to the cavity linewidth over the EO comb spectral range and therefore it can be neglected for simulations. We solve this equation numerically in the time domain using split-step method analogically to the one presented in [8].

## VIII. SUPERCONTINUUM AND SECOND-HARMONIC GENERATION IN HYBRID WAVEGUIDES

Finally, we demonstrate supercontinuum generation with combined $\chi^{(2)}$ and $\chi^{(3)}$ nonlinear optical processes using the hybrid waveguides, as shown in Fig. 8(a). A centimeter-long waveguide is pumped with an ultrafast femtosecond pulse laser at 1560 nm center wavelength, with 90 fs pulse duration, 100 MHz repetition rate, and average power up

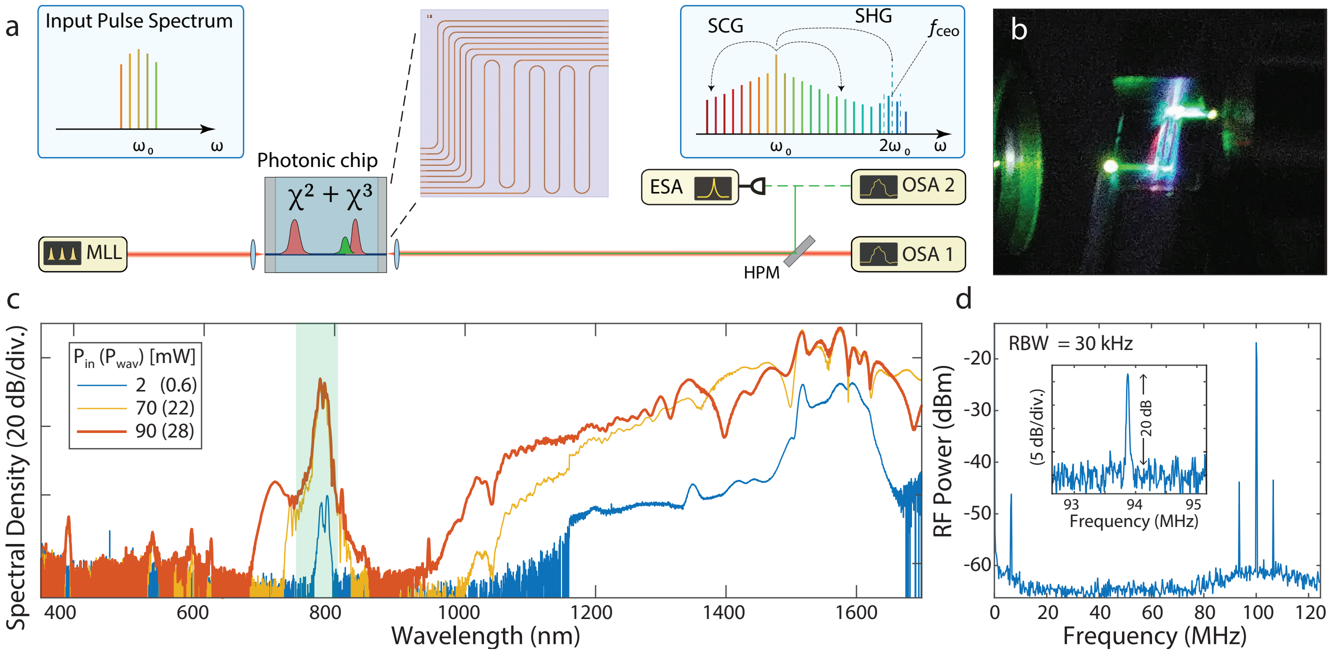


**Supplementary Figure 8: Supercontinuum generation and carrier-envelope frequency ($f_{ceo}$) measurement.** (a) Experimental schematic for supercontinuum in a $\chi^{(2)}, \chi^{(3)}$ $LiNbO_3$ waveguide, with input pulse comb spectrum on the left, and a $\chi^{(3)}$-based supercontinuum, overlapped with a $\chi^{(2)}$-based second-harmonic signal, on the right. Chip layout in the centre. Light is coupled in and out of the chip via lenses (5 dB insertion loss). MLL: Mode-locked laser, ESA: Electronic spectrum analyser. OSA: Optical spectrum analyser, HPM: spectral high-pass mirror. (b) Photo of the supercontinuum process in experiment. Blue and Green light corresponds to higher harmonic generation. (c) Total output spectrum for different incident (in waveguide) power levels $P_{\mathrm{in}}$ ($P_{\mathrm{wav}}$). (d) $f_{\mathrm{ceo}}$ beatnote and $f_{\mathrm{rep}} = 100$ MHz repetition rate beatnote, detected at $P_{\mathrm{wav}} = 28$ mW.

to 100 mW. We observe octave-spanning supercontinuum generation mediated by the $\chi^{(3)}$ nonlinearity, together with simultaneous second harmonic generation (SHG) due to optical field in $LiNbO_3$. As observed already in AlN and LNOI waveguides [9, 10], provided that the field from the supercontinuum overlaps with the SHG signal at ∼780 nm, this enables direct measurement of the carrier envelope-offset frequency $f_{\mathrm{ceo}}$ at the waveguide output with a photodetector. In Fig. 8(c), we observe isolated SHG beginning with 2 mW average power incident on the waveguide (∼ 0.6 mW in the waveguide accounting insertion loss), while supercontinuum generation is yet to take place. When the incident (on-chip) power increases to 90 mW (28 mW on chip) , we observe spectral broadening towards visible wavelengths. Importantly, a dispersive wave is formed at wavelengths around 710 nm. In this experiment, the insertion loss is higher than the one presented in the main text due to the fact, that coupling is performed using free-space lenses, not lensed fibers. As shown in Fig. 8(d), we obtain the fundamental repetition rate of the supercontinuum as well as the $f_{\mathrm{ceo}}$ in the RF spectrum, which shares similar laser noise as the seed mode-locked laser input. We emphasize that, even though the laser pumps the waveguide fundamental mode at 1560 nm, the second harmonic is generated in a higher-order waveguide mode that is phase-matched to the pumped fundamental mode. Nevertheless, it enables direct $f_{\mathrm{ceo}}$ measurement with a signal-to-noise ratio of 17 dB within a resolution bandwidth of 30 kHz, sufficient for $f_{\mathrm{ceo}}$ stabilization and optical cycle counting. Recent studies [11, 12] have shown that bare $Si_3N_4$ waveguides can simultaneously exhibit $\chi^{(3)}$ and $\chi^{(2)}$ nonlinearities, and the latter is optically induced by the photogalvanic effect and the formation of self-organized nonlinear grating. However, SHG in these bare $Si_3N_4$ waveguides suffers from the competition between the $\chi^{(3)}$ and $\chi^{(2)}$ processes, thus suffers from limited power handling capability due to the fact that SHG can be quenched by the simultaneous supercontinuum generation [12]. Our method using hybrid waveguides overcomes this challenge and enables co-generation of SHG and SCG, as the $\chi^{(3)}$ and $\chi^{(2)}$ nonlinearities are inherited from the intrinsic material properties.

## SUPPLEMENTARY TABLE 1

| Reference | Intrinsic Q-factors | Linear optical loss | $V_\pi L$ product (Tuning rate) | Insertion loss | Wafer-level fabrication | Statistical analysis |
|---|---|---|---|---|---|---|
| This work | $4\cdot10^6$ | 0.1 dB/cm | 30 V·cm[a] (42 MHz·$V^{-1}$) | 2.5 dB/facet | Yes | Yes |
| [13] | $10^7$ | 0.027 dB/cm | No data | No data | Yes | No |
| [14] | No data | No data | 6.7 V·cm | 6.5 dB/facet | No | No |
| [15] | $2.5\cdot10^6$ | No data | (500 MHz·$V^{-1}$) | No data | Yes | No |
| [16] | No data | 0.2±0.4 dB/cm | No data | 5 dB/facet | No | No |
| [17] | $1.8\cdot10^6$ | 0.27 dB/cm | No data | 1.7 dB/facet[b] | Yes | Yes |
| [18] | $7.68\cdot10^5$ | 0.2 dB/cm | 5.1 V·cm[a] | 6.5 dB/facet | Yes | No |
| [19] | No data | No data | 3.1 V·cm | No data | Yes | No |
| [20] | No data | 7 dB/cm | 3 V·cm | >10 dB/facet | Yes | No |

**Supplementary Table I:** Comparison of the main metrics described in the paper with other related publications on ridge-waveguide and heterogeneously integrated $LiNbO_3$ integrated photonics. [a] The value is estimated from the microresonator tuning rate. [b] The insertion loss value is taken from another work published by the same group [21].

## REFERENCES


[1] M. H. P. Pfeiffer, C. Herkommer, J. Liu, T. Morais, M. Zervas, M. Geiselmann, and T. J. Kippenberg, IEEE Journal of Selected Topics in Quantum Electronics **24**, 1 (2018).

[2] J. Liu, V. Brasch, M. H. P. Pfeiffer, A. Kordts, A. N. Kamel, H. Guo, M. Geiselmann, and T. J. Kippenberg, Opt. Lett. **41**, 3134 (2016).

[3] C. Wang, M. Zhang, X. Chen, M. Bertrand, A. Shams-Ansari, S. Chandrasekhar, P. Winzer, and M. Lončar, Nature **562**, 101 (2018).

[4] M. He, M. Xu, Y. Ren, J. Jian, Z. Ruan, Y. Xu, S. Gao, S. Sun, X. Wen, L. Zhou, L. Liu, C. Guo, H. Chen, S. Yu, L. Liu, and X. Cai, Nature Photonics **13**, 359 (2019), arXiv:1807.10362.

[5] James E. Toney, *Lithium Niobate Photonics* (Artech House Publishers, 2015).

[6] T. Reveyrand, in *2018 International Workshop on Integrated Nonlinear Microwave and Millimetre-wave Circuits (INMMIC)* (IEEE, 2018) pp. 1–3.

[7] A. Dutt, M. Minkov, Q. Lin, L. Yuan, D. A. B. Miller, and S. Fan, Nature Communications **10**, 3122 (2019).

[8] A. K. Tusnin, A. M. Tikan, and T. J. Kippenberg, Physical Review A **102**, 023518 (2020).

[9] D. D. Hickstein, H. Jung, D. R. Carlson, A. Lind, I. Coddington, K. Srinivasan, G. G. Ycas, D. C. Cole, A. Kowligy, C. Fredrick, S. Droste, E. S. Lamb, N. R. Newbury, H. X. Tang, S. A. Diddams, and S. B. Papp, Physical Review Applied **8**, 014025 (2017).

[10] M. Yu, B. Desiatov, Y. Okawachi, A. L. Gaeta, and M. Lončar, Optics Letters **44**, 1222 (2019).

[11] A. Billat, D. Grassani, M. H. P. Pfeiffer, S. Kharitonov, T. J. Kippenberg, and C.-S. Brès, Nature Communications **8**, 1016 (2017).

[12] D. D. Hickstein, D. R. Carlson, H. Mundoor, J. B. Khurgin, K. Srinivasan, D. Westly, A. Kowligy, I. I. Smalyukh, S. A. Diddams, and S. B. Papp, Nature Photonics **13**, 494 (2019).

[13] M. Zhang, C. Wang, R. Cheng, A. Shams-Ansari, and M. Lončar, Optica **4**, 1536 (2017).

[14] N. Boynton, H. Cai, M. Gehl, S. Arterburn, C. Dallo, A. Pomerene, A. Starbuck, D. Hood, D. C. Trotter, T. Friedmann, C. T. DeRose, and A. Lentine, Opt. Express **28**, 1868 (2020).

[15] M. Zhang, C. Wang, Y. Hu, A. Shams-Ansari, T. Ren, S. Fan, and M. Lončar, Nature Photonics **13**, 36 (2019), arXiv:1809.08638.

[16] L. Chang, M. H. P. Pfeiffer, N. Volet, M. Zervas, J. D. Peters, C. L. Manganelli, E. J. Stanton, Y. Li, T. J. Kippenberg, and J. E. Bowers, Opt. Lett. **42**, 803 (2017).

[17] K. Luke, P. Kharel, C. Reimer, L. He, M. Loncar, and M. Zhang, Opt. Express **28**, 24452 (2020).

[18] A. N. R. Ahmed, S. Shi, A. J. Mercante, and D. W. Prather, Opt. Express **27**, 30741 (2019).

[19] A. Rao, A. Patil, P. Rabiei, A. Honardoost, R. DeSalvo, A. Paolella, and S. Fathpour, Opt. Lett. **41**, 5700 (2016).

[20] S. Jin, L. Xu, H. Zhang, and Y. Li, IEEE Photonics Technology Letters **28**, 736 (2016).

[21] L. He, M. Zhang, A. Shams-Ansari, R. Zhu, C. Wang, and L. Marko, Optics Letters **44**, 2314 (2019), arXiv:1902.08969.
